# Supplementary material for: Gambling with superconducting fluctuations
Source: arXiv:1406.4723 source file (2014-12-23)
Supplement: Supplementary file 1 [file Gambling_with_superconducting_fluctuations_SUPP.pdf]

# Supplemental Material for "Gambling with superconducting fluctuations"

Marek Foltyn and Maciej Zgirski*

*Institute of Physics, Polish Academy of Sciences, al. Lotników 32/46, PL 02-668 Warszawa, Poland*

E-mail: zgirski@ifpan.edu.pl

## Random numbers

Random numbers are everywhere. In cryptography we use them to encode information, in computer simulations – to predict the behavior of various statistical systems, in gambling – to earn and lose money. Software random number generators are actually only pseudo-random because of their dependency on a seed and generating algorithm. Hardware random number generators, if properly designed, can approach the truly random number generation. Existing fast hardware random number generators (RNGs) are based on the processing of natural noise or stochastic physical phenomena. One of such devices is based on the radioactive nucleus decay.[1] Electric pulses, generated by detected particles, are counted and processed resulting in random stream of 10 kb/s. Ultra fast RNGs derive their randomness from a quantum optical physics, by detecting single photons received from attenuated and split beam of light, incident on two detectors.[2,3] Each photon detection is converted into a random bit. Such devices can generate even 2 Gb/s.[4] Commercial devices are primarily taking advantage of other physical observable, such as Johnson-Nyquist noise of resistors. Generally, amplified resistor noise is converted by comparator into a train of random-length pulses, which afterwards can be processed in many different ways in order to obtain random bits' streams.[5,6] The other examples of techniques and phenomena used for generating random bits are based on subharmonic oscillators,[7] spontaneously initiated stimulated Raman scattering,[8] turbulent electroconvection.[9] Since fluctuations are more pronounced in small physical systems it is reasonable to develop random number generators based on nanoobjects. It has been recently demonstrated that thermal oscillations of the magnetic moment in magnetic tunnel junctions[10] may be harnessed for such generation.

*To whom correspondence should be addressed

## Methods

The circuit shown in Fig. 4a consist of a pulse generator Agilent 33250A, with internal resistance 50Ω, bias resistor $R_B$=200Ω, and Aluminum Dayem nanobridge serving here as a Josephson Junction (Fig. 3). We send current pulses down the CuNi coaxial cable, guaranteeing undisturbed shape of the pulses and exhibiting low thermal conductivity suitable for cryogenic environment. To reduce external noise pulses amplitude was totally decreased by 29dB by installing four attenuators at different cryostat cooling stages. JJ voltage was multiplied 100 times by using NF LI-75A amplifier. In order to avoid mutual coupling between lines shielded twisted pairs wires were used. JJ current series responses are counted and stored by LeCroy HRO 66Zi oscilloscope. Measurements were conducted in $^3$He sorption fridge at base temperature of 350mK.

Short square pulses (with length of order of 100ns) are recommended to increase bit rate. However using twisted pairs for detection has an effect of low-pass filtering and unable to monitor fast signals. On the other hand too long pulses ($1\mu s$ or more) can overheat the junction and thereby they may require longer JJ cooling times. The remedy is to use specially tailored current waveforms consisting of a short pulse (e.g. 100ns) intended to tests a junction on its switching threshold, and sustaining pulse (e.g. $5\mu s$), with much smaller amplitude that allows for JJ switching detection. The amplitude of sustaining part is far too small to cause switching. Typical waveform shape used in our experiments is shown in Fig. 4c. To decouple from parasitic signals often emitted on 50 or 60Hz it is recommended to drive the whole experimental setup on batteries.

## Brownian motion of the ball in the tilted washboard potential (movie)

The phase difference across JJ is often visualized by a position of a ball moving in so called tilted washboard potential (Resistively and Capacitively Shounted Junction model). Such a ball undergoes the Brownian motion in the local minimum of the potential and may jump over potential barrier if its temperature-driven or quantum fluctuations are strong enough (such process is called *phase slip*). The height of the barrier is set with current flowing through the junction according to relation: $\Delta U = (2\sqrt{2}I_0\Phi_0/3\pi)(1 - I/I_0)^{3/2}$. It controls lifetime of the ball in the local minimum of the potential $\tau$ (or escape rate $\Gamma = 1/\tau$). First movie (*Brownian_fluctuations.wmv* file) shows fluctuations of the particle (phase) in the tilted washboard potential leading occasionally to phase slip (jump over the barrier). Second movie (*Phase_dynamics.wmv* file) shows fluctuating phase accross nanobridge (1D superconductor).

## Relation for escape probability for the ball subject to current pulse of duration $T$

By applying a current pulse we give the ball a chance to jump over the barrier. If lifetime in local minimum is $\tau$ then a probability for a ball to escape in short time $dt$ is $dt/\tau$. It follows that $1-dt/\tau$ is the probability that the ball does not escape in time $dt$. For current pulse of length $T$ the probability for the ball NOT to escape is $(1-dt/\tau)^{T/dt} = exp(ln(1-dt/\tau)^{T/dt})$.

On expanding logarithm around 1 ($ln(x) = 1-x$) we get $exp(-T/\tau)$. Finally, the probability for the ball to escape is $P = 1 - exp(-T/\tau)$.

Since $\tau = 1/\Gamma$ is both current and temperature dependent, escape probability can be tuned by using the feedback on current pulses e.g. by applying bisection method `http://en.wikipedia.org/wiki/Bisection_algorithm`.

## Autocorrelation of the generated sequence

In the third test stream of random bits $\{\theta_1, \theta_2, ..., \theta_i, ..., \theta_j, ..., \theta_N\}$ is analyzed for temporal correlations. We define discrete autocorrelation function in the form:

$$ac(j) = \frac{1}{n}\sum_{i=1}^{n} \theta(i) \cdot \theta(i+j) \quad (1)$$

The product in the sum should give for true random number sequence either 1 (with probability $P$=1/4) or 0 (with probability $P$=3/4). The expected value of the autocorrelation function is $< ac >= 1/4$. Autocorrelation with mean value fluctuating around 0.25 calculated for $n$=730 000 pairs. In Fig. 1 we see no evidence of frequency components.

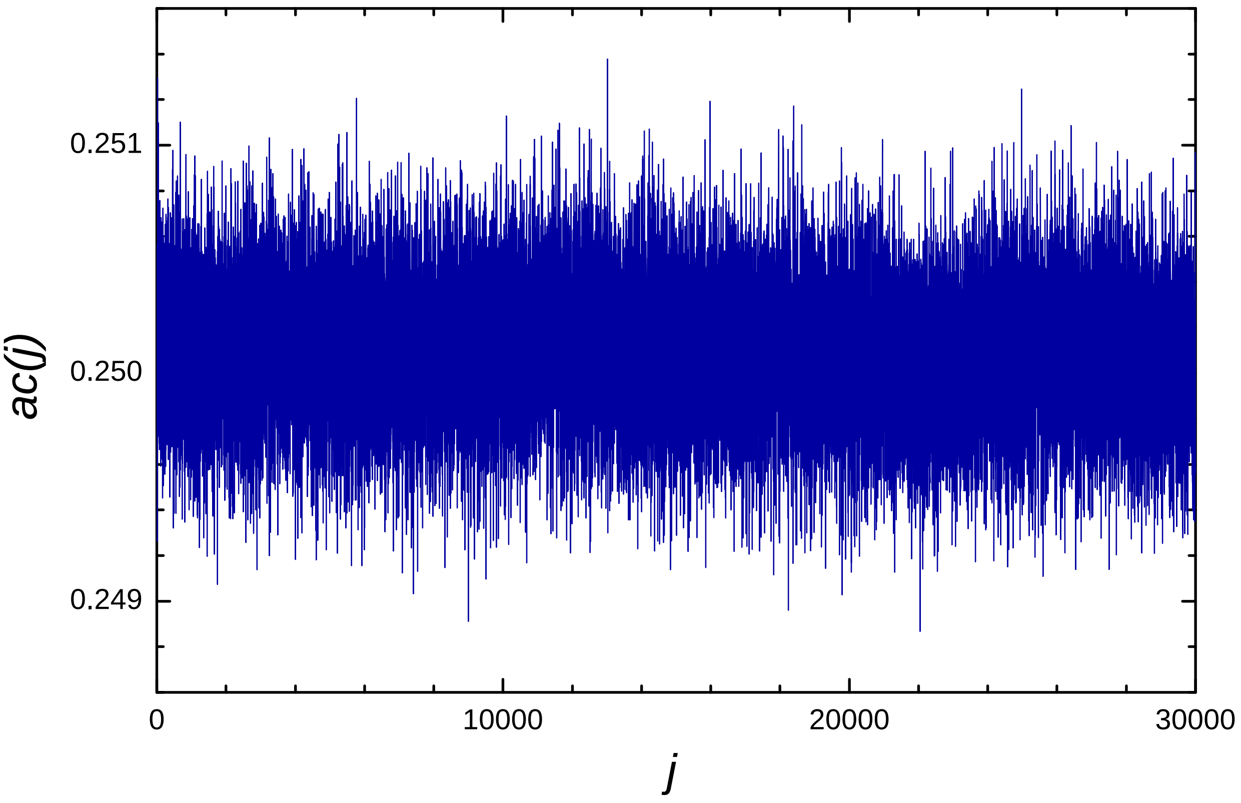


**Figure 1:** Autocorrelation of bits vs. distance between them.

## NIST Test Suite for randomness

Randomness of our data is confirmed by NIST Test Suite. Each of the fifteen tests returns one or more such called $p$-values, which determine whether the sequence is random when $p$-value is greater than 0.01. Moreover, if the sequence is random resulting $p$-values distribution must be uniform in the interval (0,1). For generated bit sequence all NIST tests give $p$-value $> 0.01$ wherein all $p$-values are uniformly distributed in the interval (0,1).

## References


(1) Isida, M.; Ikeda, Y. *Ann. Inst. Stat. Math.* **1956**, *8*, 119–126.

(2) Zbinden, H. *J. Mod. Opt.* **2000**, *47*, 595–598.

(3) Ma, H. Q.; Wang, S. M.; Zhang, D.; Chang, J. T.; Ji, L. L.; Hou, Y. X.; Wu, L. A. *Chinese Phys. Lett.* **2004**, *21*, 1961.

(4) Symul, T.; Assad, S. M.; Lam, P. K. *Appl. Phys. Lett.* **2011**, *98*, 231103.

(5) Holman, W. T.; Connelly, J. A.; Downlatabadi, A. B. *IEEE Trans. Circ. Sys. I* **1997**, *44(6)*, 521–528.

(6) Bucci, M.; Germani, L.; Luzzi, R.; Tommasino, P.; Trifiletti, A.; Varanonuovo, M. *IEEE Trans. Circ. Sys. I* **2003**, *50(Nov)*, 1373–1380.

(7) Sterzer, F. *Rev. Sci. Instrum.* **1959**, *30*, 241–243.

(8) England, D. G.; Bustard, P. J.; Moffatt, D. J.; Nunn, J.; Lausten, R.; Sussman, B. J. *Appl. Phys. Lett.* **2014**, *104*, 051117.

(9) Gleeson, J. T. *Appl. Phys. Lett.* **2002**, *81*, 1949–1951.

(10) Zhu, X.; Wu, W.; Jacobson, D. M.; Kang, S. H.; Yuen, K. H. (QUALCOMM Incorporated). Magnetic Tunnel Junction Based Random Number Generator. US Patent 0067890, 2014.
